# Supplementary material for: An Adversarial Objective for Scalable Exploration
Source: arXiv:2003.06082 source file (2020-11-11)
Supplement: Supplementary file 1 [file appendix.tex]

\begin{appendices}
\section{Experimental Details}
Additional visualizations of our results are available on our website at \href{https://sites.google.com/view/action-for-better-prediction}{https://sites.google.com/view/action-for-better-prediction}. 

Since our video prediction model only runs on a single camera's video stream, and our data collection setup had multiple cameras, our algorithm changed which camera it was using to plan after every trajectory. The hyperparameters for our planner are show in Table~\ref{tab:hparams_exploration} and ~\ref{tab:hparams_task}. The hyperparameters for our prediction model are shown in Table~\ref{tab:hyperparameters}.

\begin{wraptable}{l}{0.5\textwidth}
\centering
\begin{tabular}{|l|c|}
\hline
    Hyperparameter & Value \\
\hline\hline
    Trajectory length & 30 \\
    Robot actions per planning interval & 10 \\
    CEM iterations & 3\\
    CEM candidate actions per iteration & 200 \\
    CEM selection fraction & 0.05 \\
\hline

\end{tabular}
\caption{Hyperparameter values for the planner during exploration}
\label{tab:hparams_exploration}
\end{wraptable}

\begin{wraptable}{r}{0.5\textwidth}
\centering
\begin{tabular}{|l|c|}
\hline
    Hyperparameter & Value \\
\hline\hline
    Trajectory length & 10 \\
    Robot actions per planning interval & 10 \\
    CEM iterations & 3\\
    CEM candidate actions per iteration & 600 \\
    CEM selection fraction & 0.05 \\
\hline

\end{tabular}
\caption{Hyperparameter values for the planner during task execution}
\label{tab:hparams_task}
\end{wraptable}

\begin{wrapfigure}{l}{0.5\textwidth}
\centering
\begin{tabular}{|l|c|}
\hline
    Hyperparameter & Value \\
\hline\hline
    Schedule sampling k & 4000 \\
    Context Frames & 5 \\
    Encoder Filters & [128, 256, 256] \\
    LSTM Filters & 256 \\
    Decoder Filters & 256 \\
    Discriminator Kernel size & [3, 4, 4] \\
    Discriminator nonlinearity & Leaky ReLU \\
    Discriminator Filters & [64, 128, 256, 256] \\
    Discriminator training threshold & 0.75 \\
    GAN weight & 0.001 \\
    L1 weight & 1.0 \\
    Optimizer & Adam \cite{Kingma2015} \\
    Learning rate & 0.0001 \\
    Beta1 & 0.9 \\
    Beta2 & 0.999 \\
\hline
\end{tabular}
\caption{Prediction model hyperparameter values.}
\label{tab:hyperparameters}
\end{wrapfigure}

\end{appendices}
